# Supplementary material for: Learning to Import through Production Networks
Source: arXiv:2405.13422 source file (2025-02-24)
Supplement: Supplementary file 1 [file tbl_Network_BasicInfo_NotIncluded.tex]

%
% Such constructed dataset contains information about on average 10.05 million connections among  firms per year (2010 - 2014) among an average 831525 firms.

% \begin{table}
%     \centering
%     \begin{tabular}{|c|c|c|c|}
%         Year & Number of links &  Number of firms &AverageValueLink\\
%         \hline
%         2010 & 11593279 &  845276 & 74928.26 \\
%         \hline
%         2011 &11200026  &  864986 & 78086.21\\
%         \hline
%         2012 & 10266703 & 848885 & 109908.40 \\
%         \hline
%         2013 & 9896132 & 829947 &  82995.49\\
%         \hline
%         2014 & 9576451  &  768532 & 85430.89\\
%         \hline
%     \end{tabular}
%     \caption{Some information about network. Not to be included in the final version}
%     \label{tab:my_label}
% \end{table}

% \begin{table}
%     \centering
%     \begin{tabular}{|c|c|c|c|}
%         Year & Number of links &  Number of firms &AverageValueLink\\
%         \hline
%         2010 &8736804  &  611996 &  84108.77 \\
%         \hline
%         2011 & 9101097  &  611996 &  86067.78\\
%         \hline
%         2012 & 8758302 & 611996 & 121270.22 \\
%         \hline
%         2013 & 8489903 & 611996 & 88812.95\\
%         \hline
%         2014 &  8273487   &  611996 &  89147.18\\
%         \hline
%     \end{tabular}
%     \caption{Some information about network. Only firms appearing in all years.  Not to be included in the final version}
%     \label{tab:my_label}
%\end{table}

% There are  firms that appear in the network in each year 2010--2014. 
